# Supplementary material for: GenAI Against Humanity: Nefarious Applications of Generative Artificial Intelligence and Large Language Models
Source: arXiv:2310.00737 source file (2024-01-22)
Supplement: Supplementary file 1 [file sec-appendix.tex]

\appendix

\section*{Appendix: Background}
The rapid evolution of Large Language Models (LLMs) has revolutionized the landscape of natural language processing and understanding. Beginning with the seminal work on the Transformer architecture by Vaswani et al. \citeAppendix{transformer}, a series of breakthroughs have been achieved in the domain of LLMs. The GPT series, starting with the foundational work by Radford et al. \citeAppendix{gpt}, followed by subsequent advancements in GPT-2 \citeAppendix{gpt2}, GPT-3 \citeAppendix{gpt3}, and the recent GPT-4 \citeAppendix{gpt4}, have showcased the power of generative pre-training. Furthermore, the integration of visual elements with LLMs \citeAppendix{visualchatgpt} --a growing trend in Generative AI (GenAI) models (e.g., DALL-E 3)\footnote{OPEN AI's DALL-E 3: \url{https://openai.com/dall-e-3}}-- underscores the expanding horizons of these models beyond the mere text. As GenAI and LLMs continue to evolve, it is imperative to understand their capabilities, malicious applications, and associated challenges they present.

\section*{A Taxonomy of Abuse and Malicious Applications of GenAI and LLMs}

\begin{table}[h]
\centering
\caption{Summary of LLM-related problem domains and associated issues}
\label{tab:llm_summary}
\begin{tabularx}{\textwidth}{lXl}
\toprule
\textbf{Problem Domain} & \textbf{Issue} & \textbf{References} \\
\midrule
Security Risks in LLMs & Generative AI Risks & \citeAppendix{barrett2023identifying} \\
& Jailbreaking LLMs & \citeAppendix{lapid2023open} \\
& LLMs and Malware & \citeAppendix{derner2023ratgpt, charan2023text} \\

\midrule
Vulnerabilities and Attacks on LLMs & Backdoor Attacks  & \citeAppendix{yang2023comprehensive} \\
& Instruction-based Vulnerabilities & \citeAppendix{xu2023instructions} \\
\midrule
Ethical Implications & Ethical Challenges and Guidelines & \citeAppendix{zhou2023ethical, ferrara2023fairness, ferrara2023should} \\
& Security and Ethical Implications of ChatGPT & \citeAppendix{derner2023beyond} \\

\midrule
Safety \& Alignment  & Benchmarking LLM Safety and Robustness & \citeAppendix{qiu2023latent, ferrara2023butterfly} \\
& Defense Against Adversarial Prompts & \citeAppendix{kumar2023certifying} \\
& Behavioral Alignment of LLMs & \citeAppendix{wolf2023fundamental, kumar2023certifying} \\
\midrule
Societal Impacts of LLMs & Release Strategies and Societal Implications & \citeAppendix{openai2019release} \\
& LLMs and Harmful Content Generation & \citeAppendix{mcguffie2020radicalization} \\
& Auto-Radicalization \& Self-Radicalization & \citeAppendix{wang2023identifying} \\
% & Alienation & \citeAppendix{} \\
\midrule
LLM Misuse \& Nefarious Applications & AI-Powered Botnets on Social Media & \citeAppendix{ferrara2016rise, yang2023anatomy, ferrara2023social} \\
& Propaganda \& Influence Operations & \citeAppendix{pierri2023propaganda, haider2023detecting, ezzeddine2022characterizing} \\
& Disinformation \& Misinformation & \citeAppendix{sharma2022construction} \\
& Spam, Phishing, \& Impersonation & \citeAppendix{ferrara2019history} \\
\bottomrule
\end{tabularx}
\end{table}

The advent of Large Language Models (LLMs) has brought about a paradigm shift in the realm of artificial intelligence, particularly in natural language processing and understanding. While their capabilities have been harnessed for numerous beneficial applications, the power of LLMs has also opened the door to various forms of abuse and malicious applications. This section provides an extensive exploration of the darker side of LLMs, highlighting the myriad ways in which they can be and have been misused.

\begin{enumerate}[label=\textbf{\arabic*.}]
    \item \textbf{Misinformation and Disinformation Campaigns}:
    \begin{itemize}
        \item LLMs can generate highly convincing fake news, misleading narratives, or propaganda. These can be used to manipulate public opinion, interfere with elections, or incite unrest.
        \item They can also be employed to create fake reviews, testimonials, or comments on online platforms, misleading consumers or swaying perceptions.
    \end{itemize}
    
    \item \textbf{Automated Cyberattacks}:
    \begin{itemize}
        \item LLMs can be trained to craft phishing emails or messages that are highly personalized and convincing, increasing the success rate of such attacks.
        \item They can assist in automating certain stages of cyberattacks, such as reconnaissance, by scraping and processing vast amounts of data to identify potential vulnerabilities or targets.
    \end{itemize}
    
    \item \textbf{Malicious Content Generation}:
    \begin{itemize}
        \item LLMs can be used to generate offensive, harmful, or radicalizing content, which can then be disseminated on social media or other platforms.
        \item They can produce extremist propaganda, hate speech, or other forms of divisive content that can bypass traditional content filters.
    \end{itemize}
    
    \item \textbf{Software Vulnerability Exploitation}:
    \begin{itemize}
        \item LLMs can be employed to identify software vulnerabilities or to craft exploits for known vulnerabilities.
        \item They can assist in obfuscating malicious code, making it harder for traditional security systems to detect.
    \end{itemize}
    
    \item \textbf{Identity Theft and Social Engineering}:
    \begin{itemize}
        \item By processing available data, LLMs can impersonate individuals, crafting messages or responses that seem genuine.
        \item They can be used in advanced social engineering attacks, manipulating individuals into divulging confidential information or performing actions against their best interests.
    \end{itemize}
    
    \item \textbf{Deepfakes and Multimedia Manipulation}:
    \begin{itemize}
        \item While primarily associated with video and image manipulation, LLMs can assist in generating realistic audio deepfakes, impersonating voices or creating entirely fabricated conversations.
        \item They can also generate scripts or narratives for deepfake videos, enhancing their believability.
    \end{itemize}
    
    \item \textbf{Financial Fraud}:
    \begin{itemize}
        \item LLMs can be employed in stock market manipulation by generating fake news or rumors that can influence stock prices.
        \item They can assist in crafting sophisticated financial scams, creating fake investment opportunities, or impersonating financial advisors.
    \end{itemize}
    
    \item \textbf{Backdoor Attacks and Hidden Triggers}:
    \begin{itemize}
        \item Malicious actors can introduce hidden triggers during the training phase of LLMs. When these triggers are activated, the model can produce predefined malicious outputs.
        \item Such backdoors can be used to manipulate the model's behavior in unintended ways, potentially causing harm or facilitating other attacks.
    \end{itemize}
    
    \item \textbf{Data Privacy Concerns}:
    \begin{itemize}
        \item There's a potential risk of LLMs inadvertently generating outputs that contain sensitive or private information, especially if they were exposed to such data during their training.
        \item This can lead to unintentional data leaks or breaches of privacy.
    \end{itemize}
    
    \item \textbf{Bias Amplification and Discrimination}:
    \begin{itemize}
        \item If not carefully managed, LLMs can perpetuate or even amplify societal biases present in their training data.
        \item This can result in discriminatory outputs, reinforcing stereotypes, or marginalizing certain groups.
    \end{itemize}
\end{enumerate}

\begin{table}[h!]
    \centering \footnotesize
    \begin{tabularx}{\textwidth}{|p{2.2cm}|X|X|}
        \hline
        \textbf{Application} & \textbf{Example} & \textbf{Proof-of-Concept} \\
        \hline
        Deepfake Video Creation & Combining LLMs with video generation tools can produce realistic "deepfake" videos where public figures appear to say or do things they never did. & Using an LLM to script a fabricated speech and then using a video generation tool to create a video of a world leader "delivering" that speech. \\
        \hline
        Fake Audio Recordings & LLMs can be used to script conversations, which can then be turned into realistic audio recordings using voice synthesis tools, potentially leading to misinformation or blackmail scenarios. & Generating a fake phone call between two celebrities discussing a controversial topic. \\
        \hline
        Synthetic Identity Theft & Combining LLMs with image generation tools can create entirely synthetic identities, complete with fake personal histories, photos, and other credentials. & Creating a fake online persona with a detailed backstory, photos, and social media presence, which can then be used for scams or misinformation campaigns. \\
        \hline
        Manipulated News Footage & LLMs can script fake news segments, which can then be turned into realistic news footage using video generation tools, potentially spreading false information or propaganda. & Generating a fake news segment about a fabricated natural disaster or political event. \\
        \hline
        Augmented Reality (AR) Misinformation & Combining LLMs with AR tools can create misleading augmented reality experiences, overlaying false information or visuals onto the real world. & Designing an AR application that falsely labels landmarks or provides misleading historical information to users. \\
        \hline
        Fake Social Media Content Generation & LLMs can be used to script posts, tweets, or comments, while image generation tools create accompanying visuals, leading to large-scale misinformation campaigns on social media platforms. & Orchestrating a coordinated social media campaign with fake user profiles, posts, and images to influence public opinion on a particular topic. \\
        \hline
        Misleading Medical Imagery & Combining LLMs with medical image generation tools can produce fake medical images, potentially leading to misdiagnoses or fraudulent research. & Generating a fake MRI or X-ray image showing a medical condition that isn't present. \\
        \hline
        Fake Historical Footage & LLMs can script historical events, and video generation tools can create footage that appears to be from the past, potentially altering perceptions of history. & Creating a video that falsely depicts a historical event, such as a meeting between two historical figures who never actually met. \\
        \hline
        Automated Adversarial Attacks & LLMs can be used to design strategies for adversarial attacks on AI systems, while other generative tools create the necessary inputs (like images) to execute these attacks. & Designing and executing an attack on a facial recognition system using generated images that confuse the AI. \\
        \hline
        Fake Product Demonstrations & Combining LLMs with video generation tools can create fake product demonstrations or reviews, misleading consumers about a product's capabilities or performance. & Generating a video that shows a product performing a function it can't actually perform in reality. \\
        \hline
         Generating Offensive or Harmful Art & Generative AI models can produce art, music, or literature that is offensive, promotes hate, or is otherwise harmful. & Using a generative art model and subtly guiding it with prompts that lead to the creation of artwork with hidden offensive symbols or messages. \\
        \hline
    \end{tabularx}
    \caption{Malicious Applications of LLMs in Combination with Other Generative AI Systems (e.g., Image or Video Generation).}
\end{table}

\bibliographystyleAppendix{ACM-Reference-Format}
\bibliographyAppendix{chatgpt,genai}
